# Supplementary material for: Charge density waves and stripes in quarter metals of graphene heterostructures
Source: arXiv:2510.20816 ancillary file (2026-08-15)
Supplement: Supplementary file 1 [file Supplementary_Stripe_Graphene.pdf]

# Supplemental Material:
# Charge-density waves and stripes in quarter metals of graphene heterostructures

Sk Asrap Murshed[1] and Bitan Roy[1]

[1]*Department of Physics, Lehigh University, Bethlehem, Pennsylvania, 18015, USA*

(Dated: October 23, 2025)

Supplemental material includes details of the (a) generalized two-band Hamiltonian for chirally-stacked $n$ layer, including rhombohedral multilayer, Bernal bilayer, and monolayer, graphene up to $n = 6$, where $n$ is number of layers [see Sec. S1], (b) derivation of the matrix representation of valley-coherent charge-density wave (VC-CDW) order in monolayer graphene [see Sec. S2], and (c) details of the mean field calculation capturing a competition between VC-CDW and anomalous Hall order in the quarter-metal [see Sec. S3 and Fig. S1].

## S1. GENERALIZED HAMILTONIAN FOR MULTILAYER GRAPHENE

We start the discussion with the derivation of a low-energy effective two-band model for chirally-stacked $n$ layer graphene (containing a total of $2n$ number of bands at the bare level) that includes monolayer ($n = 1$), Bernal bilayer ($n = 2$), and rhombohedral multi-layer ($n \geq 3$) graphene, by integrating out $2n - 2$ high-energy bands for $n \geq 2$. We construct the minimal model Hamiltonian for free fermions, which includes in-plane hopping $t_0$ between the sites from two complementary sublattices, the direct hopping $t_p$ between sites from different sublattices living in the adjacent layers, and both momentum dependent ($t_1$) and momentum independent ($t_2$) hopping amplitudes, responsible for the trigonal warping, between the sites from two different sublattices in the nearest-neighbor layers and next-nearest-neighbor layers, respectively. See Fig. 1 of the main manuscript for reference. In the following, the hopping amplitudes $t_0$ and $t_1$ are replaced with $\alpha_0 = \left(\sqrt{3}/2\right) t_0$ and $\alpha_1 = \left(\sqrt{3}/2\right) t_1$, respectively, obtained by keeping only the linear in momentum ($\boldsymbol{k}$) terms in the Bloch Hamiltonian around the respective valleys. The values of the band parameters are listed in Table I for all discussed graphene systems, which are measured in units of $t_0$ and throughout we set the lattice spacing $a = 1$. Our effective model also incorporates an applied electric potential, which results in a sagging of the bands, stemming from the external electric displacement field ($D$) in the stacking direction. The layer-specific electric potential on the $m$th layer is defined as $V_{nm}$, where $n$ denotes the total number of layers in the graphene heterostructure with $m \leq n$ and

$$V_{nm} = V\left(\frac{1}{2} - \frac{m-1}{n-1}\right). \tag{S1}$$

The electric displacement field is $D = V/[(n-1)d]$, where $d$ is the separation between adjacent layers.

The tight-binding Hamiltonian for graphene multilayers is divided into four parts, which are highlighted with color-coded dashed boxes in the following subsections. The unboxed section represents the segment of the tight binding Hamiltonian operative on two low-energy sites and it is denoted as $H_{LL}$. The red dashed box, on the other hand, represents the portion of the Hamiltonian acting on all the high-energy sites and it is denoted as $H_{HH}$. Finally, the blue dashed boxes include the coupling between the low-energy and high-energy sites. They are denoted as $H_{LH}$ and $H_{HL}$, which satisfy the relation $H_{LH} = H^{\dagger}_{HL}$. The renormalized Hamiltonian, captured by an effective two-band model in all the systems, obtained after integrating out the high-energy sites, is given by the generic form

$$H^{n}_{eff} = H_{LL}(\boldsymbol{k}) - H_{LH}H^{-1}_{HH}H_{HL}(\boldsymbol{k}) = \begin{pmatrix} D & X \\ X^{\star} & -D \end{pmatrix}(\boldsymbol{k}) = \boldsymbol{\eta}\cdot\boldsymbol{F}(\boldsymbol{k}). \tag{S2}$$

The explicit form of the vector $\boldsymbol{F}(\boldsymbol{k})$ depends on the band parameters, $n$, and momentum $\boldsymbol{k}$ measured about a given valley momentum. For concreteness, in this section we focus near the valley at $+\mathbf{K}$. The set of Pauli matrices $\{\eta_\nu\}$ operates on the sublattice or layer index, where $\nu = 0, \cdots, 3$. The planar components of $\boldsymbol{F}(\boldsymbol{k})$, namely $F_1(\boldsymbol{k})$ and $F_2(\boldsymbol{k})$, can be expressed in terms of the spherical harmonics of appropriate orders in a particular system. The detailed forms and corresponding spherical harmonic functions are listed in Table II. By contrast, $F_3(k)$ is a function expressed in term of even-powers of $|\boldsymbol{k}|$ and always equal to $D$ from Eq. (S2). We now follow this general procedure to arrive at the effective low-energy model in all the systems one by one, starting with the monolayer graphene.

| Band Parameters | Values in units of $t_0$ | | | | | |
|---|---|---|---|---|---|---|
| | $n=1$ [1] | $n=2$ [2, 3] | $n=3$ [4, 5] | $n=4$ [6, 7] | $n=5$ [8, 9] | $n=6$ [10] |
| $\alpha_0$ | 0.866 | 0.866 | 0.866 | 0.866 | 0.866 | 0.866 |
| $\alpha_1$ | 0 | 0.087 | −0.109 | −0.078 | −0.096 | −0.096 |
| $t_p$ | 0 | 0.133 | 0.159 | 0.123 | 0.137 | 0.137 |
| $t_2$ | 0 | 0 | −0.003 | −0.003 | −0.003 | −0.003 |
| $V$ | – | 0.034 − 0.080 | 0.067 − 0.137 | 0.270 − 0.330 | 0.131 − 0.158 | 0.523 − 0.589 |

Table I. Band parameters for chirally-stacked $n$ layer graphene heterostructures that include monolayer ($n=1$), Bernal bilayer ($n=2$), and rhombohedral multi-layer ($n \geq 3$) graphene. In the first column, the top two band parameters are $\alpha_0 = \left(\sqrt{3}/2\right) t_0$ and $\alpha_1 = \left(\sqrt{3}/2\right) t_1$, where $t_0$ is the in-plane nearest-neighbor hopping amplitude and $t_1$ is the out-of-plane hopping amplitude between the adjacent layers, responsible for the momentum-dependent trigonal warping. The rest of the band parameters in the first column are the direct or dimer hopping between nearest-neighbor layers $t_p$, next-to-nearest inter-layer momentum independent trigonal warping hopping $t_2$, and applied electric potential across the layers $V$, yielding the quarter-metal phase and accounting for the effects of perpendicular electric displacement field. See Sec. S1 for details. Here, all the parameters are expressed in units of $t_0$ and we choose the lattice spacing $a$ to be unity. The rest of the columns show the values of these band parameters for individual graphene layers, denoted by their total number of layers $n$.

### A. Monolayer Graphene ($n = 1$)

We start with the assumption that there is a staggered potential applied between two sublatices of the monolayer graphene. In this case, the system contains two bands and there exists no high-energy band. Therefore, the tight-binding Hamiltonian, which is also an effective two-band Hamiltonian in the spinor basis $\Psi = \left[c_{a_1}, c_{b_1}\right]^\top$, where $c_{a_1}$ ($c_{b_1}$) is the fermionic annihilation operator on the sites of the $A$ ($B$) sublattice on layer 1, takes the form

$$H_{\text{monolayer}} = \begin{pmatrix} V_{11} & \alpha_0 k^\star \\ \alpha_0 k & -V_{11} \end{pmatrix}, \tag{S3}$$

where $k = k_x + i k_y$ and $k^\star = k_x - i k_y$, and these notations are used hereon. Therefore, the form of the $\boldsymbol{F}(\boldsymbol{k})$ vector is

$$\boldsymbol{F}(\boldsymbol{k}) = \left(\alpha_0 k_x, \alpha_0 k_y, V_{11}\right). \tag{S4}$$

### B. Bernal Bilayer Graphene ($n = 2$)

The tight binding Hamiltonian for Bernal bilayer graphene (BBLG), written in the spinor basis of $\Psi = \left[c_{a_1}, c_{b_1}, c_{a_2}, c_{b_2}\right]^\top$, where $a_1$ and $b_2$ corresponds to low-energy sites, $a_2$ and $b_1$ are high-energy sites, and $c_{a_i}$ ($c_{b_i}$) is the fermionic annihilation operator on the sites of sublattice $a_i(b_i)$ in the $i$th layer, reads as

$$H_{\text{bilayer}} = \begin{pmatrix} V_{21} & \alpha_0 k^\star & \alpha_4 k^\star & \alpha_1 k \\ \alpha_0 k & V_{21} & t_p & \alpha_4 k^\star \\ \alpha_4 k & t_p & -V_{21} & \alpha_0 k^\star \\ \alpha_1 k^\star & \alpha_4 k & \alpha_0 k & -V_{21} \end{pmatrix}. \tag{S5}$$

Following the same procedure discussed earlier in the section and using Eq. (S2), the explicit forms of $X$ and $D$ are

$$X = \left(k_x + i k_y\right) \alpha_1 - \frac{\alpha_0^2 \left(k_x - i k_y\right)^2}{t_p} \quad \text{and} \quad D = V_{21}\left(1 - \frac{\alpha_0^2}{t_p^2 + V_{21}^2}\left(k_x^2 + k_y^2\right)\right) = F_3(\boldsymbol{k}), \tag{S6}$$

| Momentum harmonics | Components | Explicit form in terms of $k_x, k_y$ | Explicit form in terms of $k, \phi_k$ |
|---|---|---|---|
| $\boldsymbol{p}$ | $(p_1, p_2)$ | $(k_x, k_y)$ | $k\,(\cos[\phi_k], \sin[\phi_k])$ |
| $\boldsymbol{d}$ | $(d_1, d_2)$ | $(k_x^2 - k_y^2, 2k_xk_y)$ | $k^2(\cos[2\phi_k], \sin[2\phi_k])$ |
| $\boldsymbol{f}$ | $(f_1, f_2)$ | $(k_x(k_x^2 - 3k_y^2), k_y(3k_x^2 - k_y^2))$ | $k^3(\cos[3\phi_k], \sin[3\phi_k])$ |
| $\boldsymbol{g}$ | $(g_1, g_2)$ | $(k_x^4 - 6k_x^2k_y^2 + k_y^4, 4k_xk_y(k_x^2 - k_y^2))$ | $k^4(\cos[4\phi_k], \sin[4\phi_k])$ |
| $\boldsymbol{h}$ | $(h_1, h_2)$ | $(k_x^5 - 10k_x^3k_y^2 + 5k_xk_y^4, 5k_x^4k_y - 10k_x^2k_y^3 + k_y^5)$ | $k^5(\cos[5\phi_k], \sin[5\phi_k])$ |
| $\boldsymbol{i}$ | $(i_1, i_2)$ | $(k_x^6 - 15k_x^4k_y^2 + 15k_x^2k_y^4 - k_y^6, 6k_x^5k_y - 20k_x^3k_y^3 + 6k_xk_y^5)$ | $k^6(\cos[6\phi_k], \sin[6\phi_k])$ |

Table II. First six spherical harmonics of planar momentum in $d = 2$. The first column describes the order of the harmonics and the second column shows the vector representation of the harmonics in two dimensions. Finally, third (fourth) column shows explicit forms of the harmonics vector components in terms of $k_x$ and $k_y$ ($k = \sqrt{k_x^2 + k_y^2}$ and $\phi_k = \tan^{-1}(k_y/k_x)$).

and the remaining components of $\boldsymbol{F(k)}$ are given by (see Table II)

$$F_1(\boldsymbol{k}) = \alpha_1 p_1 - \frac{\alpha_0^2}{tp} d_1 \quad \text{and} \quad F_2(\boldsymbol{k}) = -\alpha_1 p_2 - \frac{\alpha_0^2}{t_p} d_2. \tag{S7}$$

### C. Rhombohedral Trilayer Graphene ($n = 3$)

The tight binding Hamiltonian for ABC or rhombohedral trilayer graphene (RTLG) in the spinor basis of $\Psi = [c_{a_1}, c_{b_1}, c_{a_2}, c_{b_2}, c_{a_3}, c_{b_3}]^\top$ with $a_1$ and $b_3$ representing low-energy sites, and where $c_{a_i}(c_{b_i})$ is the fermionic annihilation operator on the sites of the sublattice $a_i(b_i)$ in the $i$th layer, is given by

$$H_{\text{trilayer}} = \begin{pmatrix} V_{31} & \alpha_0 k^\star & \alpha_4 k^\star & \alpha_1 k & 0 & t_2 \\ \alpha_0 k & V_{31} & t_p & \alpha_4 k^\star & 0 & 0 \\ \alpha_4 k & t_p & 0 & \alpha_0 k^\star & \alpha_4 k^\star & \alpha_1 k \\ \alpha_1 k^\star & \alpha_4 k & \alpha_0 k & 0 & t_p & \alpha_4 k^\star \\ 0 & 0 & \alpha_4 k & t_p & -V_{31} & \alpha_0 k^\star \\ t_2 & 0 & \alpha_1 k^\star & \alpha_4 k & \alpha_0 k & -V_{31} \end{pmatrix}. \tag{S8}$$

Therefore, $X$ and $D$ from Eq. (S2) take the forms

$$X = t_2 + \frac{-2\alpha_0\alpha_1 t_p \left(k_x^2 + k_y^2\right) + \alpha_0^3 \left(k_x - ik_y\right)^3}{t_p^2} \quad \text{and} \quad D = \frac{V_{31}\left(\alpha_0^2 k^2 \left(V_{31}^2 - \alpha_0^2 k^2\right) + t_p^4\right)}{\alpha_0^2 V_{31}^2 k^2 + t_p^4} = F_3(\boldsymbol{k}), \tag{S9}$$

and the remaining components of $\boldsymbol{F(k)}$ can be written as (see Table II)

$$F_1(\boldsymbol{k}) = \frac{1}{t_p^2}\left(f_1\alpha_0^3 + t_2 t_p^2 - 2t_p\alpha_0\alpha_1\left(p_1^2 + p_2^2\right)\right) \quad \text{and} \quad F_2(\boldsymbol{k}) = \frac{1}{t_p^2} f_2 \alpha_0^3. \tag{S10}$$

### D. Rhombohedral Tetralayer Graphene ($n = 4$)

After performing an analysis, which is similar to the one shown in the previous subsections, the tight binding Hamiltonian for ABCA-stacked tetralayer graphene in the spinor basis of $\Psi = [c_{a_1}, c_{b_1}, c_{a_2}, c_{b_2}, c_{a_3}, c_{b_3}, c_{a_4}, c_{b_4}]^\top$ with $c_{a_i}\,(c_{b_i})$ as the annihilation operator on the sites of the $a_i(b_i)$ sublattice in the $i$th layer, and $a_1$, $b_4$ acting as effective low-energy sites and the rest of the sites acting as the high-energy sites, reads as

| Systems | $X_{\text{low}}$ | $X_{\text{high}}$ | $k^\star_{02}$ | $k^\star_{12}$ | $k^\star_{23}$ | $k^\star_{34}$ | $k^\star_{45}$ | $k^\star_{56}$ |
|---|---|---|---|---|---|---|---|---|
| Monolayer ($n=1$) | $k$ | $k$ | - | - | - | - | - | - |
| Bilayer ($n=2$) | $k$ | $k^2$ | - | 0.0154 | - | - | - | - |
| Trilayer ($n=3$) | $k^0$ | $k^3$ | 0.0458 | - | 0.0462 | - | - | - |
| Tetralayer ($n=4$) | $k$ | $k^4$ | - | 0.7117 | 0.0043 | 0.0384 | - | - |
| Pentalayer ($n=5$) | $k$ | $k^5$ | - | 0.0116 | 0.2819 | 0.0132 | 0.0702 | - |
| Hexalayer ($n=6$) | $k^0$ | $k^6$ | 0.0574 | - | 0.0263 | 0.0241 | 0.0211 | 0.0877 |

Table III. Information on the critical momentum points in graphene multilayers along the momentum axis. Here, we provide explicit values of $k^\star_{mn}$ from Fig. S1 for every system. The first column specifies the system, whereas the second and the third columns state the lowest and highest order of $k$ present in corresponding $X$ from Eq. (S2), respectively. The rest of the columns provide detailed information on values of corresponding critical $k^\star_{mn}$ points. As an example, for bilayer graphene system, the value of critical point $k^\star_{12}$ is 0.0154, implying that for $k > 0.0154$ ($k < 0.0154$), the $k^2$ ($k$) term dominates over the $k$ ($k^2$) term.

$$H_{\text{tetralayer}} = \begin{pmatrix} V_{41} & \alpha_0 k^\star & \alpha_4 k^\star & \alpha_1 k & 0 & t_2 & 0 & 0 \\ \alpha_0 k & V_{41} & t_p & \alpha_4 k^\star & 0 & 0 & 0 & 0 \\ \alpha_4 k & t_p & V_{42} & \alpha_0 k^\star & \alpha_4 k^\star & \alpha_1 k & 0 & t_2 \\ \alpha_1 k^\star & \alpha_4 k & \alpha_0 k & V_{42} & t_p & \alpha_4 k^\star & 0 & 0 \\ 0 & 0 & \alpha_4 k & t_p & -V_{42} & \alpha_0 k^\star & \alpha_4 k^\star & \alpha_1 k \\ t_2 & 0 & \alpha_1 k^\star & \alpha_4 k & \alpha_0 k & -V_{42} & t_p & \alpha_4 k^\star \\ 0 & 0 & 0 & 0 & \alpha_4 k & t_p & -V_{41} & \alpha_0 k^\star \\ 0 & 0 & t_2 & 0 & \alpha_1 k^\star & \alpha_4 k & \alpha_0 k & -V_{41} \end{pmatrix}. \tag{S11}$$

Therefore, $X$ and $D = D_{\text{num}}/D_{denom} = F_3(\boldsymbol{k})$ are given by

$$\begin{aligned} X &= -\frac{-3\alpha_1\alpha_0^2 t_p (k_x - ik_y)^2 (k_x + ik_y) + 2\alpha_0 t_2 t_p^2 (k_x - ik_y) + \alpha_1^2 t_p^2 (k_x + ik_y)^2 + \alpha_0^4 (k_x - ik_y)^4}{t_p^3}, \\ D_{\text{num}} &= \alpha_0^4 \left(k_x^2 + k_y^2\right)^2 \left(-V_{42} t_p^2 + V_{41}^3 + 2V_{42}^2 V_{41}\right) + \alpha_0^2 V_{42} \left(k_x^2 + k_y^2\right)\left(V_{41}V_{42} - t_p^2\right)\left(t_p^2 + 2V_{41}^2 + V_{42}^2\right) \\ &+ \alpha_0^6 V_{41} \left(-\left(k_x^2 + k_y^2\right)^3\right) + V_{41}\left(t_p^2 - V_{41}V_{42}\right)^2 \left(t_p^2 + V_{42}^2\right), \\ \text{and} \quad D_{\text{denom}} &= 2\alpha_0^2 V_{41} V_{42} \left(k_x^2 + k_y^2\right)\left(t_p^2 - V_{41}V_{42}\right) + \alpha_0^4 V_{41}^2 \left(k_x^2 + k_y^2\right)^2 + \left(t_p^2 - V_{41}V_{42}\right)^2 \left(t_p^2 + V_{42}^2\right). \end{aligned} \tag{S12}$$

Finally, the form of the remaining components of the $\boldsymbol{F}(\boldsymbol{k})$ vector can be expressed as (see Table II)

$$\begin{aligned} F_1(\boldsymbol{k}) &= -\left(2\frac{t_2\alpha_0}{t_p} p_1 + \frac{\alpha_0^4}{t_p^3} g_1 - 3\frac{\alpha_0^2\alpha_1}{t_p^2}\left(p_1^2 + p_2^2\right) p_1 + \frac{\alpha_1^2}{t_p} d_1\right) \\ \text{and } F_2(\boldsymbol{k}) &= -\left(2\frac{t_2\alpha_0}{t_p} p_2 + \frac{\alpha_0^4}{t_p^3} g_2 - 3\frac{\alpha_0^2\alpha_1}{t_p^2}\left(p_1^2 + p_2^2\right) p_2 - \frac{\alpha_1^2}{t_p} d_2\right). \end{aligned} \tag{S13}$$

### E. Rhombohedral Pentalayer Graphene ($n = 5$)

The tight binding Hamiltonian for rhombohedral pentalayer graphene in the spinor basis of $\Psi = [c_{a_1}, c_{b_1}, c_{a_2}, c_{b_2}, c_{a_3}, c_{b_3}, c_{a_4}, c_{b_4}, c_{a_5}, c_{b_5}]^\top$ with $c_{a_i}(c_{b_i})$ as the fermionic annihilation operator on the sites of sub-

lattice $a_i$ ($b_i$) in the $i$th layer, and $a_1$ and $b_5$ acting as low-energy sites and the rest (namely, $b_1$, $a_2$, $b_2$, $a_3$, $b_3$, $a_4$, $b_4$, and $a_5$) as high-energy sites, is given by

$$H_{\text{pentalayer}} = \begin{pmatrix} V_{51} & \alpha_0 k^\star & \alpha_4 k^\star & \alpha_1 k & 0 & t_2 & 0 & 0 & 0 & 0 \\ \alpha_0 k & V_{51} & t_p & \alpha_4 k^\star & 0 & 0 & 0 & 0 & 0 & 0 \\ \alpha_4 k & t_p & V_{52} & \alpha_0 k^\star & \alpha_4 k^\star & \alpha_1 k & 0 & t_2 & 0 & 0 \\ \alpha_1 k^\star & \alpha_4 k & \alpha_0 k & V_{52} & t_p & \alpha_4 k^\star & 0 & 0 & 0 & 0 \\ 0 & 0 & \alpha_4 k & t_p & 0 & \alpha_0 k^\star & \alpha_4 k^\star & \alpha_1 k & 0 & t_2 \\ t_2 & 0 & \alpha_1 k^\star & \alpha_4 k & \alpha_0 k & 0 & t_p & \alpha_4 k^\star & 0 & 0 \\ 0 & 0 & 0 & 0 & \alpha_4 k & t_p & -V_{52} & \alpha_0 k^\star & \alpha_4 k^\star & \alpha_1 k \\ 0 & 0 & t_2 & 0 & \alpha_1 k^\star & \alpha_4 k & \alpha_0 k & -V_{52} & t_p & \alpha_4 k^\star \\ 0 & 0 & 0 & 0 & 0 & 0 & \alpha_4 k & t_p & -V_{51} & \alpha_0 k^\star \\ 0 & 0 & 0 & 0 & t_2 & 0 & \alpha_1 k^\star & \alpha_4 k & \alpha_0 k & -V_{51} \end{pmatrix}. \tag{S14}$$

After performing the band projection procedure stated above in Eq. (S2), the form of the effective two-band model Hamiltonian components with $D = D_{\text{num}}/D_{denom} = F_3(\boldsymbol{k})$ are

$$\begin{aligned} X &= \left(3\alpha_0^2 t_2 t_p^2 (k_x - ik_y)^2 + 3\alpha_1^2 \alpha_0 t_p^2 (k_x - ik_y)(k_x + ik_y)^2 \right. \\ &- \left. 2\alpha_1 t_p (k_x + ik_y)\left(t_2 t_p^2 + 2\alpha_0^3 (k_x - ik_y)^3\right) + \alpha_0^5 (k_x - ik_y)^5\right)/t_p^4, \\ D_{\text{num}} &= \alpha_0^6 \left(k_x^2 + k_y^2\right)^3 \left(-V_{52} t_p^2 + V_{51}^3 + 2V_{52}^2 V_{51}\right) + \alpha_0^4 V_{52}\left(2V_{51}^2 + V_{52}^2\right)\left(k_x^2 + k_y^2\right)^2 \left(t_p^2 - V_{51}V_{52}\right) \\ &+ \alpha_0^2 V_{52}\left(k_x^2 + k_y^2\right)\left(-2V_{51}^2 V_{52}^2 t_p^2 + t_p^6 + V_{51}^3 V_{52}^3\right) + \alpha_0^8 V_{51}\left(-\left(k_x^2 + k_y^2\right)^4\right) + V_{51} t_p^4 \left(t_p^2 - V_{51}V_{52}\right)^2, \\ \text{and} \quad D_{\text{denom}} &= 2\alpha_0^4 V_{51} V_{52} \left(k_x^2 + k_y^2\right)^2 \left(t_p^2 - V_{51}V_{52}\right) + \alpha_0^2 V_{52}^2 \left(k_x^2 + k_y^2\right)\left(t_p^2 - V_{51}V_{52}\right)^2 \\ &+ \alpha_0^6 V_{51}^2 \left(k_x^2 + k_y^2\right)^3 + t_p^4 \left(t_p^2 - V_{51}V_{52}\right)^2. \end{aligned} \tag{S15}$$

As we have discussed above, $F_1(\boldsymbol{k})$ and $F_2(\boldsymbol{k})$ for pentalayer are respectively given by (see Table II)

$$\begin{aligned} F_1(\boldsymbol{k}) &= \left(-2\frac{t_2\alpha_1}{t_p}p_1 + 3\frac{t_2\alpha_0^2}{t_p^2}d_1 + \frac{\alpha_0^5}{t_p^4}h_1 - 4\frac{\alpha_0^3\alpha_1}{t_p^3}(p_1^2+p_2^2)d_1 + 3\frac{\alpha_0\alpha_1^2}{t_p^2}(p_1^2+p_2^2)p_1\right) \\ \text{and} \quad F_2(\boldsymbol{k}) &= \left(2\frac{t_2\alpha_1}{t_p}p_2 + 3\frac{t_2\alpha_0^2}{t_p^2}d_2 + \frac{\alpha_0^5}{t_p^4}h_2 - 4\frac{\alpha_0^3\alpha_1}{t_p^3}(p_1^2+p_2^2)d_2 - 3\frac{\alpha_0\alpha_1^2}{t_p^2}(p_1^2+p_2^2)p_2\right). \end{aligned} \tag{S16}$$

### F. Rhombohedral Hexalayer Graphene ($n = 6$)

The tight binding Hamiltonian for ABC-stacked hexalayer graphene with $a$ sublattice from the bottom layer and $b$ sublattice from the top layer acting as low energy states, and in the spinor basis of $\Psi = [c_{a_1}, c_{b_1}, c_{a_2}, c_{b_2}, c_{a_3}, c_{b_3}, c_{a_4}, c_{b_4}, c_{a_5}, c_{b_5}, c_{a_6}, c_{b_6}]^\top$ with $c_{a_i}(c_{b_i})$ as the fermionic annihilation operator on the sites of sublattice $a_i(b_i)$ in the $i$th layer, is defined as

$$H_{\text{hexalayer}} = \begin{pmatrix} V_{61} & \alpha_0 k^\star & \alpha_4 k^\star & \alpha_1 k & 0 & t_2 & 0 & 0 & 0 & 0 & 0 & 0 \\ \alpha_0 k & V_{61} & t_p & \alpha_4 k^\star & 0 & 0 & 0 & 0 & 0 & 0 & 0 & 0 \\ \alpha_4 k & t_p & V_{62} & \alpha_0 k^\star & \alpha_4 k^\star & \alpha_1 k & 0 & t_2 & 0 & 0 & 0 & 0 \\ \alpha_1 k^\star & \alpha_4 k & \alpha_0 k & V_{62} & t_p & \alpha_4 k^\star & 0 & 0 & 0 & 0 & 0 & 0 \\ 0 & 0 & \alpha_4 k & t_p & V_{63} & \alpha_0 k^\star & \alpha_4 k^\star & \alpha_1 k & 0 & t_2 & 0 & 0 \\ t_2 & 0 & \alpha_1 k^\star & \alpha_4 k & \alpha_0 k & V_{63} & t_p & \alpha_4 k^\star & 0 & 0 & 0 & 0 \\ 0 & 0 & 0 & 0 & \alpha_4 k & t_p & -V_{63} & \alpha_0 k^\star & \alpha_4 k^\star & \alpha_1 k & 0 & t_2 \\ 0 & 0 & t_2 & 0 & \alpha_1 k^\star & \alpha_4 k & \alpha_0 k & -V_{63} & t_p & \alpha_4 k^* & 0 & 0 \\ 0 & 0 & 0 & 0 & 0 & 0 & \alpha_4 k & t_p & -V_{62} & \alpha_0 k^\star & \alpha_4 k^\star & \alpha_1 k \\ 0 & 0 & 0 & 0 & t_2 & 0 & \alpha_1 k^\star & \alpha_4 k & \alpha_0 k & -V_{62} & t_p & \alpha_4 k^* \\ 0 & 0 & 0 & 0 & 0 & 0 & 0 & 0 & \alpha_4 k & t_p & -V_{61} & \alpha_0 k^\star \\ 0 & 0 & 0 & 0 & 0 & 0 & t_2 & 0 & \alpha_1 k^\star & \alpha_4 k & \alpha_0 k & -V_{61} \end{pmatrix}. \tag{S17}$$

Therefore, components of the effective two-band model Hamiltonian with $D = D_{\text{num}}/D_{denom} = F_3(\boldsymbol{k})$ are

$$\begin{aligned} X &= \frac{1}{t_p^5}\big(5\alpha_1\alpha_0^4 t_p\,(k_x - ik_y)^4\,(k_x+ik_y) - 6\alpha_1^2\alpha_0^2 t_p^2\,(k_x^2+k_y^2)^2 + 2\alpha_0 t_2 t_p^2\big(3\alpha_1 t_p\,(k_x^2+k_y^2) \\ &- 2\alpha_0^2\,(k_x-ik_y)^3\big) + \alpha_1^3 t_p^3\,(k_x+ik_y)^3 + \alpha_0^6\left(-(k_x-ik_y)^6\right) - t_2^2 t_p^4\big), \\ D_{\text{num}} &= t_p^8\left(\alpha_0^2 V_{62}\left(k_x^2+k_y^2\right) - 2V_{62}V_{61}^2 + V_{63}\left(V_{63}-2V_{62}\right)V_{61}\right) + t_p^6\big(\alpha_0^4 V_{63}\left(k_x^2+k_y^2\right)^2 \\ &- \alpha_0^2\left(V_{61}V_{62}^2 - V_{63}^2V_{62} + 2\left(V_{61}^2 - V_{62}V_{61} + V_{62}^2\right)V_{63}\right)\left(k_x^2+k_y^2\right) + V_{61}V_{62}\big(-2V_{63}^3 \\ &+ \left(V_{62}-2V_{61}\right)V_{63}^2 + 4V_{61}V_{62}V_{63} + V_{61}^2V_{62}\big)\big) + t_p^4\big(-\alpha_0^6 V_{63}\left(k_x^2+k_y^2\right)^3 \\ &+ \alpha_0^4\big(V_{63}^3 - V_{62}V_{63}^2 + 2\left(V_{61}^2 - V_{62}V_{61} + V_{62}^2\right)V_{63} \\ &+ V_{61}V_{62}^2\big)\left(k_x^2+k_y^2\right)^2 + \alpha_0^2 V_{63}\big(2V_{61}V_{62}\left(V_{61}-V_{62}\right)^2 - 2\left(V_{61}^2+V_{62}^2\right)V_{63}^2 \\ &+ V_{62}\left(V_{62}-2V_{61}\right)\left(V_{62}-V_{61}\right)V_{63}\big)\left(k_x^2+k_y^2\right) + V_{61}V_{62}^2V_{63}\big(V_{63}^3 + 2V_{61}\left(2V_{63}-V_{62}\right)V_{63} \\ &+ V_{61}^2\left(V_{63}-2V_{62}\right)\big)\big) + t_p^2\left(V_{62}^2 - \alpha_0^2\left(k_x^2+k_y^2\right)\right)\left(V_{63}V_{61}^3\left(\alpha_0^2\left(2V_{62}-V_{63}\right)\left(k_x^2+k_y^2\right)\right.\right. \\ &+ \left.\left. V_{62}\left(V_{62}-2V_{63}\right)V_{63}\right) - 2V_{62}V_{61}^2\left(V_{63}^2 - \alpha_0^2\left(k_x^2+k_y^2\right)\right)^2 + \alpha_0^2V_{63}V_{61}\,\times \right. \\ &\quad \left(k_x^2+k_y^2\right)\left(\alpha_0^2\left(V_{63}-2V_{62}\right)\left(k_x^2+k_y^2\right) - V_{62}\left(V_{62}-2V_{63}\right)V_{63}\right) + V_{62}\left(k_x^2+k_y^2\right)\times \\ &\quad \left(\alpha_0 V_{63}^2 - \alpha_0^3\left(k_x^2+k_y^2\right)\right)^2\big) + V_{61}\left(V_{61}^2 - \alpha_0^2\left(k_x^2+k_y^2\right)\right)\left(V_{62}^2 - \alpha_0^2\left(k_x^2+k_y^2\right)\right)^2\times \\ &\quad \left(V_{63}^2 - \alpha_0^2\left(k_x^2+k_y^2\right)\right)^2 + V_{61}t_p^{10}, \\ \text{and}\quad D_{\text{denom}} &= -2\alpha_0^6 V_{61}\left(k_x^2+k_y^2\right)^3\left(V_{61}\left(V_{62}^2+V_{63}^2\right) - V_{62}t_p^2\right) + \alpha_0^4\left(k_x^2+k_y^2\right)^2\big(\left(V_{62}^2 + 2V_{61}V_{63}\right)t_p^4 \\ &+ V_{61}\big(-2V_{62}^3 2V_{63}\left(V_{61}+2V_{63}\right)V_{62} + V_{61}V_{63}^2\big)t_p^2 + V_{61}^2\left(V_{62}^4 + 4V_{63}^2V_{62}^2 + V_{63}^4\right)\big) \\ &- 2\alpha_0^2 V_{63}\left(k_x^2+k_y^2\right)\left(t_p^2 - V_{61}V_{62}\right)\left(t_p^2 - V_{62}V_{63}\right)\left(\left(V_{61}-V_{62}\right)t_p^2 + V_{61}\left(V_{62}^2+V_{63}^2\right)\right) \\ &+ \alpha_0^8 V_{61}^2\left(k_x^2+k_y^2\right)^4 + \left(t_p^2 - V_{61}V_{62}\right)^2\left(t_p^2 - V_{62}V_{63}\right)^2\left(t_p^2+V_{63}^2\right). \end{aligned} \tag{S18}$$

The remaining components of $\boldsymbol{F}(\boldsymbol{k})$ are (see Table II)

$$\begin{aligned} F_1(\boldsymbol{k}) &= \Big(-\frac{t_2^2}{t_p} - \frac{\alpha_0^6}{t_p^5}i_1 + 5\frac{\alpha_0^4\alpha_1}{t_p^4}\left(p_1^2+p_2^2\right)f_1 - 6\frac{\alpha_0^2\alpha_1^2}{t_p^3}\left(p_1^2+p_2^2\right)^2 + \frac{\alpha_1^3}{t_p^2}f_1 - 4\frac{t_2\alpha_0^3}{t_p^3}f_1 + 6\frac{t_2\alpha_0\alpha_1}{t_p^2}\left(p_1^2+p_2^2\right)\Big) \\ \text{and}\; F_2(\boldsymbol{k}) &= \left(-\frac{\alpha_0^6}{t_p^5}i_2 + 5\frac{\alpha_0^4\alpha_1}{t_p^4}\left(p_1^2+p_2^2\right)f_2 - \frac{\alpha_1^3}{t_p^2}f_2 - 4\frac{t_2\alpha_0^3}{t_p^3}f_2\right). \end{aligned} \tag{S19}$$

## S2. VALLEY-COHERENT CHARGE-DENSITY WAVE (VC-CDW) IN MONOLAYER GRAPHENE

The tight binding Hamiltonian for graphene with an added onsite potential term $V(r_i)$ that corresponds to VC-CDW order is given by

$$H = -t \sum_{\langle i,j \rangle} \left( a_i^\dagger b_j + \text{h.c} \right) + \sum_i V\left(\boldsymbol{r}_i\right) c_i^\dagger c_i. \tag{S20}$$

Here, $t$ is a uniform hopping amplitude between the nearest-neighbor sites belonging to the sublattices $a$ at $\boldsymbol{r}_i$ and $b$ at $\boldsymbol{r}_j$ in monolayer graphene, and $\langle \cdots \rangle$ restricts the summation to the nearest-neighbor sites. For now, we neglect the second term. Then, after performing a Fourier transformation, the tight binding Hamiltonian can be rewritten in terms of the Bloch Hamiltonian $H = \psi^\dagger h(\boldsymbol{q}) \psi$ in the basis of $\psi = [\psi_a, \psi_b]^\top(\boldsymbol{q})$ where $\psi_a(\boldsymbol{q})$, and $\psi_b(\boldsymbol{q})$ are the fermionic annihilation operators for sites $a$ and $b$ with crystal momentum $\boldsymbol{q}$, respectively. The form of $h(\boldsymbol{q})$ becomes

$$h(\boldsymbol{q}) = \begin{pmatrix} 0 & f(\boldsymbol{q}) \\ f^\star(\boldsymbol{q}) & 0 \end{pmatrix} \tag{S21}$$

with $f(q) = -t \sum_i \exp\left(i\boldsymbol{q} \cdot \boldsymbol{\delta_i}\right)$ , where $\delta_i$ are the vectors connecting a site from one sublattice to the three nearest-neighbor sites, belonging to the other sublattice. The explicit form of $\boldsymbol{\delta_i}$ are

$$\delta_1 = \frac{a}{2}\left(1, \sqrt{3}\right), \qquad \delta_2 = \frac{a}{2}\left(1, -\sqrt{3}\right), \qquad \text{and} \quad \delta_3 = a\left(-1, 0\right). \tag{S22}$$

One can expand the Hamiltonian around valley points $\mathbf{K}$ and $\mathbf{K}' = -\mathbf{K}$ to study low energy physics of monolayer graphene. Expanding $f(\boldsymbol{q})$ around $\mathbf{K}$ with $\boldsymbol{q} = \mathbf{K} + \boldsymbol{k}$, where $|\boldsymbol{k}| \ll |\mathbf{K}|$, and making a rotation by $\pi/6$ in the $(k_x, k_y)$ plane, we obtain

$$f\left(\mathbf{K} + k\right) = -\frac{\sqrt{3}ta}{2}\left(k_x - ik_y\right). \tag{S23}$$

Therefore, around valley $\mathbf{K}$, the Hamiltonian becomes $h(k) = v_{\text{F}}\left(\eta_x k_x + \eta_y k_y\right)$ with $v_{\text{F}} = -\sqrt{3}ta/2$. Subsequently, inclusion of valley degrees of freedom in the low-energy tight binding Hamiltonian within the new basis of $\Psi = [\psi_{a,\mathbf{K}}, \psi_{b,\mathbf{K}}, \psi_{a,\mathbf{K}'}, \psi_{b,\mathbf{K}'}]^\top$ is defined as

$$h(k) = v_{\text{F}}\left(\Gamma_{31} k_x + \Gamma_{02} k_y\right), \tag{S24}$$

where $\Gamma_{\mu\nu} = \tau_\mu \otimes \eta_\nu$, and the newly introduced set of Pauli matrices $\{\tau_\nu\}$ operate on the valley index with $\nu = 0, \cdots, 3$. Here, one should notice that under $\mathbf{K} \to \mathbf{K}'$ transformation, $(k_x, k_y)$ goes to $(-k_x, k_y)$.

Let us focus on the onsite potential from Eq. (S20). It can form the VC-CDW order, implying that the resulting state is a coherent superposition of fermionic states near both valleys ($\mathbf{K}$ and $\mathbf{K}'$), which mixes the valleys while leaving the sublattices unchanged. Therefore, one can explicitly write such states as

$$\Psi_{a_i} = e^{i\mathbf{K}\cdot\mathbf{r}_i}\, \psi_{a_i,\mathbf{K}}\left(\mathbf{r}_i\right) + e^{i\mathbf{K}'\cdot\mathbf{r}_i}\, \psi_{a_i,\mathbf{K}'}\left(\mathbf{r}_i\right) \quad \text{and} \quad \Psi_{b_i} = e^{i\mathbf{K}\cdot\mathbf{r}_i}\, \psi_{b_i,\mathbf{K}}\left(\mathbf{r}_i\right) + e^{i\mathbf{K}'\cdot\mathbf{r}_i}\, \psi_{b_i,\mathbf{K}'}\left(\mathbf{r}_i\right). \tag{S25}$$

Here we also assume that $V\left(r_{b_i}\right) = V\left(r_{a_i} + \boldsymbol{\delta_i}\right) = e^{i\phi} V\left(r_{a_i}\right)$, where $\phi$ is the phase difference between two sublattices. The form of onsite potential for $a$ sublattices becomes

$$V(r) a_i^\dagger a_i = V\left(r\right)[e^{-i\mathbf{K}\cdot\mathbf{r}_i}\, \psi^\dagger_{a_i,\mathbf{K}}\left(\mathbf{r}_i\right) + e^{-i\mathbf{K}'\cdot\mathbf{r}_i}\, \psi^\dagger_{a_i,\mathbf{K}'}\left(\mathbf{r}_i\right)][e^{i\mathbf{K}\cdot\mathbf{r}_i}\, \psi_{a_i,\mathbf{K}}\left(\mathbf{r}_i\right) + e^{i\mathbf{K}'\cdot\mathbf{r}_i}\, \psi_{a_i,\mathbf{K}'}\left(\mathbf{r}_i\right)]. \tag{S26}$$

The terms like $\psi^\dagger_{a_i,\mathbf{K}}(\mathbf{r}_i)\psi_{a_i,\mathbf{K}}(\mathbf{r}_i)$ and $\psi^\dagger_{a_i,\mathbf{K}'}(\mathbf{r}_i)\psi_{a_i,\mathbf{K}'}(\mathbf{r}_i)$ contribute to valley unmixed states and are represented by matrices like $\Gamma_{0,0/3}$. Here, we only consider the valley mixing terms. With the basis as $\Psi = [\psi_{a_i,\mathbf{K}}, \psi_{b_i,\mathbf{K}}, \psi_{a_i,\mathbf{K}'}, \psi_{b_i,\mathbf{K}'}]^\top$, such terms take the form

$$\sum_i V\left(r_i\right) c_i^\dagger c_i = V(r)[\cos(\mathbf{G}\cdot\mathbf{r})\tau_1 + \sin(\mathbf{G}\cdot\mathbf{r})\tau_2] \otimes \begin{pmatrix} 1 & 0 \\ 0 & e^{i\phi} \end{pmatrix}. \tag{S27}$$

Here $\mathbf{G} = \mathbf{K} - \mathbf{K}' \equiv 2\mathbf{K}$ and depending on the phase difference between sublatices, $e^{i\phi} = +1$ ( in phase) and $-1$ ( $\pi$ out of phase), which transform in the sublattice sector as $\eta_0$ and $\eta_3$, respectively. Therefore, one finds the following one-to-one correspondences between the potential terms in the last equation and the resulting matrix representations

$$\Gamma_{1,0/3} \leftrightarrow \cos\left(\mathbf{G}\cdot\boldsymbol{r}\right), \quad \text{and} \quad \Gamma_{2,0/3} \leftrightarrow \sin\left(\mathbf{G}\cdot\boldsymbol{r}\right). \tag{S28}$$

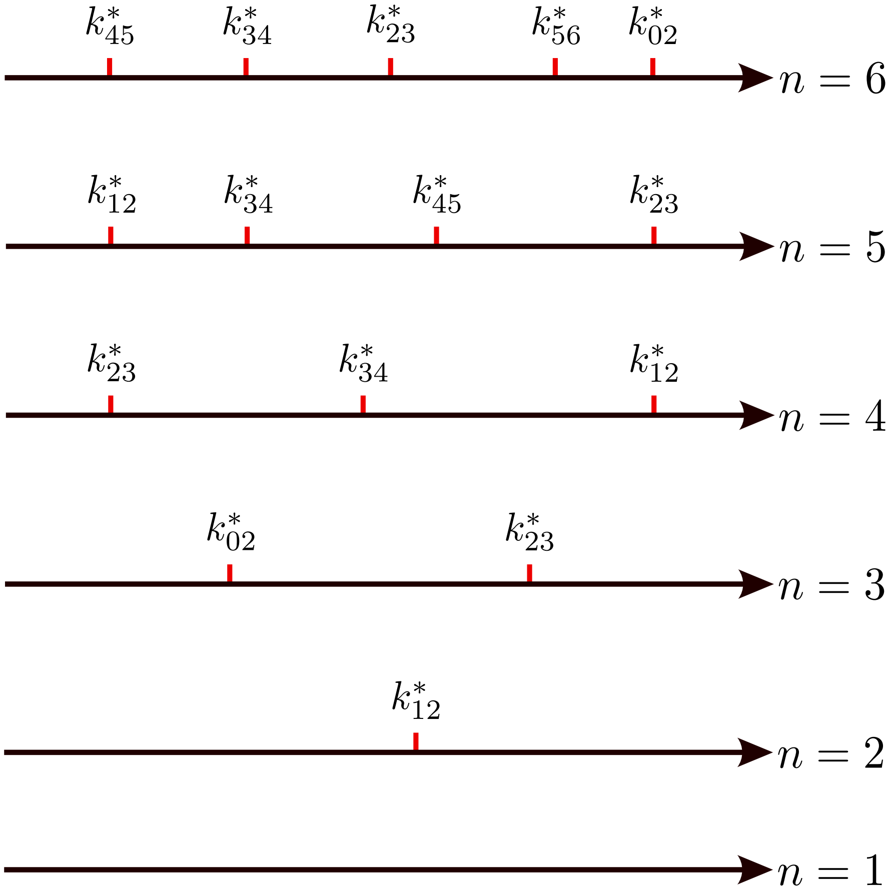


Figure S1. Schematic location of the critical momentum $k^\star_{mn}$ for all the graphene multilayers discussed here, denoted with the corresponding number of layers ($n$). For monolayer, $X$ from Eq. (S2) only depends on the first order of momentum resulting in no critical point on the $k$ axis, whereas the rest of the systems have non-trivial $k^\star_{mn}$ points according to their specific form of $X$. The critical points, denoted by $k^\star_{mn}$, represent specific momenta that separate regions where different $k$-dependent terms dominate. Namely, for $k > k^\star_{mn}$ ($k < k^\star_{mn}$), the $k^n$ ($k^m$) term dominates over the $k^m$ ($k^n$) term. See Table III

Notice that the VC-CDW order does not mix two sublattices. Therefore, in chirally-stacked multi-layer graphene systems, where the sites belonging to two sublattices reside on the top and bottom layers (see Fig. 1 of the main manuscirpt), the above construction generalizes immediately, as shown in Fig. 2(a) of the main manuscript.

## S3. MEAN FIELD CALCULATION

This section is dedicated to the mean field calculation capturing the competition between the VC-CDW and anomalous Hall order, both of which can give rise to a quarter-metal. The inclusion of a repulsive on-site Hubbard interaction induces an antiferromagnetic order parameter, which lifts the spin degeneracy of layer-polarized (by adding electric potential) graphene heterostructure and leads to a spin-polarized half-metallic phase. Subsequently, the incorporation of an anamolous Hall order with amplitude $\Delta_1$, as well as the VC-CDW order with amplitude $\Delta_2$ lifts the valley degeneracy, resulting in a spin and valley-polarized quarter-metal state. The effective single-particle Hamiltonian in the presence of these two orders in a spin-polarized system is

$$H = \Gamma_{01} d_{01} + \Gamma_{02} d_{02} + \Gamma_{31} d_{31} + \Gamma_{32} d_{32} + \Gamma_{03} d_3 + \Delta_1 \Gamma_{33} + \Delta_2 \Gamma_{10}. \qquad \text{(S29)}$$

The exact form of $d_{ij}$ can be retrieved from the explicit form of $\boldsymbol{F(k)}$ in Eq. (S2). Here, $\Gamma_{0i}$ and $\Gamma_{3i}$ (with $i = 1, 2$) are introduced and they are associated with the corresponding functions $d_{0i}$ and $d_{3i}$. The function $d_{0i}$ contains only the even powers of $k_x$ and $k_y$, whereas $d_{3i}$ has all the odd powers of $k_x$ and $k_y$. The energy spectrum of this Hamiltonian

is

$$E_\tau^\rho = \tau \left( d_{01}^2 + d_{02}^2 + d_{31}^2 + d_{32}^2 + d_3^2 + \Delta_1^2 + \Delta_2^2 + 4\rho \left[ \left( d_{01} d_{31} + d_{02} d_{32} + \Delta_1 d_3 \right)^2 + \Delta_2^2 \left( d_{01}^2 + d_{02}^2 + d_3^2 \right) \right] \right)^{1/2}, \quad \text{(S30)}$$

where $\tau, \rho = \pm$. Notice that $\tau = \pm$ represent the conduction and valence band, where as $\rho = \pm$ indicates the lifting of the residual valley degeneracy.

The geometry of the Fermi ring plays a crucial role in determining the effective interactions that give rise to various ordered phases. Therefore, the chemical potential must be explicitly included in the free energy at finite temperature. Under the mean-field approximation, the free energy density in the presence of these two orders, yieding quarter metal at temperature $T$ is defined as

$$F = \frac{\Delta_1^2}{2g_1} + \frac{\Delta_2^2}{2g_2} - k_B T \sum_{\tau,\rho} \int \frac{d^2k}{(2\pi)^2} \ln \left[ \cosh \left( \frac{|E_\tau^\rho - \mu|}{2k_B T} \right) \right], \quad \text{(S31)}$$

where $k_B$ is the Boltzmann constant. Minimizing the free energy density with respect to $\Delta_1$ and $\Delta_2$ distinctively, we find the coupled gap equations

$$\frac{1}{g_1} = \int \frac{d^2k}{(2\pi)^2} \sum_{\tau,\rho} \frac{1}{E_\tau^\rho} \left( 1 + \rho \frac{d_3/\Delta_1}{[1+x^2]^{1/2}} \right) \tanh \left( \frac{|E_\tau^\rho - \mu|}{2k_B T} \right)$$

$$\text{and} \quad \frac{1}{g_2} = \int \frac{d^2k}{(2\pi)^2} \sum_{\tau,\rho} \frac{1}{E_\tau^\rho} \left( 1 + \rho \frac{(d_{01}^2 + d_{02}^2 + d_3^2)^{1/2}/\Delta_2}{[1+1/x^2]^{1/2}} \right) \tanh \left( \frac{|E_\tau^\rho - \mu|}{2k_B T} \right), \quad \text{(S32)}$$

respectively, where $x^2 = \Delta_2^2 \left( d_{01}^2 + d_{02}^2 + d_3^2 \right) / \left( d_{01} d_{31} + d_{02} d_{32} + \Delta_1 d_3 \right)^2$. For numerical calculation, we set $k_B = 1$.

We apply a systematic technique to improve calculation efficiency. The $X$ component from Eq. (S2) contains multiple $k$-dependent terms, each of which dominates within a specific range of momentum. Accordingly, we divide the $k$-integration into distinct intervals, and within each interval consider only the dominant power of $k$ in $X$ while neglecting the other terms. In order to take into account the sagging effect (due to displacement electric fields), we only consider the lowest and highest orders of $k$ in $D_{\text{num}}$ and $D_{\text{denom}}$. The value of the critical points, which define the boundaries between these $k$-space regions, can be derived systematically. In Table III, the values of the critical ($k_{mn}^\star$) points are listed for all discussed systems. One can also get a qualitative idea of our scheme from Fig. S1, where $k_{mn}^\star$ indicates a boundary between two regions in $k$ space dominated by $k^m$ and $k^n$ terms, respectively. We also want to mention that every region in $k$ space can have either $(\Gamma_{01}, \Gamma_{32})$ or $(\Gamma_{31}, \Gamma_{02})$ terms from Eq. (S29), which further simplifies our calculations.

---


[1] P. R. Wallace, The Band Theory of Graphite, Phys. Rev. **71**, 622 (1947).

[2] L. M. Zhang, Z. Q. Li, D. N. Basov, and M. M. Fogler, Z. Hao and M. C. Martin, Determination of the electronic structure of bilayer graphene from infrared spectroscopy, Phys. Rev. B **78**, 235408 (2008).

[3] H. Zhou, L. Holleis, Y. Saito, L. Cohen, W. Huynh, C. L. Patterson, F. Yang, T. Taniguchi, K. Watanabe, and A. F. Young, Isospin magnetism and spin-polarized superconductivity in Bernal bilayer graphene, Science **375**, 774 (2022).

[4] F. Zhang, B. Sahu, H. Min, and A. H. MacDonald, Band structure of *ABC*-stacked graphene trilayers, Phys. Rev. B **82**, 035409 (2010).

[5] H. Zhou, T. Xie, A. Ghazaryan, T. Holder, J. R. Ehrets, E. M. Spanton, T. Taniguchi, K. Watanabe, E. Berg, M. Serbyn, and A. F. Young, Half and quarter metals in rhombohedral trilayer graphene, Nature (London) **598**, 429 (2021).

[6] G. Parra-Martínez, A. Jimeno-Pozo, V. T. Phong, H. Sainz-Cruz, D. Kaplan, P. Emanuel, Y. Oreg, P. A. Pantaleón, J. Á. Silva-Guillén, and F. Guinea, Band Renormalization, Quarter Metals, and Chiral Superconductivity in Rhombohedral Tetralayer Graphene, Phys. Rev. Lett. **135**, 136503 (2025).

[7] T. Han, Z. Lu, Z. Hadjri, L. Shi, Z. Wu, W. Xu, Y. Yao, A. A. Cotten, O. S. Sedeh, H. Weldeyesus, J. Yang, J. Seo, S. Ye, M. Zhou, H. Liu, G. Shi, Z. Hua, K. Watanabe, T. Taniguchi, P. Xiong, D. M. Zumbühl, L. Fu, and L. Ju, Signatures of Chiral Superconductivity in Rhombohedral Graphene, Nature **643**, 654 (2025).

[8] Z. Dong, A. S. Patri, and T. Senthil, Theory of Quantum Anomalous Hall Phases in Pentalayer Rhombohedral Graphene Moiré Structures, Phys. Rev. Lett. **133**, 206502 (2024).

[9] T. Han, Z. Lu, G. Scuri, J. Sung, J. Wang, T. Han, K. Watanabe, T. Taniguchi, H. Park, and L. Ju, Correlated insulator and Chern insulators in pentalayer rhombohedral-stacked graphene, Nat. Nanotechnol. **19**, 181 (2024).

[10] E. Morissette, P. Qin, H.-T. Wu, N. J. Zhang, R. Q. Nguyen, K. Watanabe, T. Taniguchi, and J. I. A. Li, Striped Superconductor in Rhombohedral Hexalayer Graphene, arXiv:2504.05129 (2025).
